# Supplementary material for: Optical properties and exciton transfer between N-heterocyclic carbene iridium (III) complexes for blue light-emitting diode applications from first principles
Source: arXiv:2312.12160 ancillary file (2024-02-23)
Supplement: Supplementary file 1 [file SM.pdf]

# Supplementary Material for "Optical properties and exciton transfer between N-heterocyclic carbene iridium (III) complexes for blue light-emitting diode applications from first principles"

Irina V. Lebedeva[1] and Joaquim Jornet-Somoza[1, 2]
[1)] *Nano-Bio Spectroscopy Group and ETSF, Universidad del País Vasco, CFM CSIC-UPV/EHU, 20018 San Sebastián, Spain*
[2)] *Max Planck Institute for the Structure and Dynamics of Matter and Center for Free-Electron Laser Science, Luruper Chaussee 149, 22761 Hamburg, Germany*

(*Electronic mail: liv_ira@hotmail.com (I. V. Lebedeva), j.jornet.somoza@gmail.com (J. Jornet-Somoza))

## EFFECT OF EXCHANGE-CORRELATION FUNCTIONAL ON COMPUTED SPECTRA

The absorption spectra computed using different exchange-correlation functionals (LDA[1], PBE[2] and PBE0[3]) for the same structure of the NHC blue emitter geometrically optimized using the PBE0 functional are shown in Fig. S1. The scissor operators are applied to the spectra computed using the LDA and PBE functionals. With these corrections, positions of the peaks corresponding to the first optical transitions are very close for all three functionals. The oscillator strengths of the first peaks for the LDA and PBE functionals are underestimated by 20 – 40%. Therefore, the LDA and PBE functionals can be used for qualitative studies of the exciton transfer.

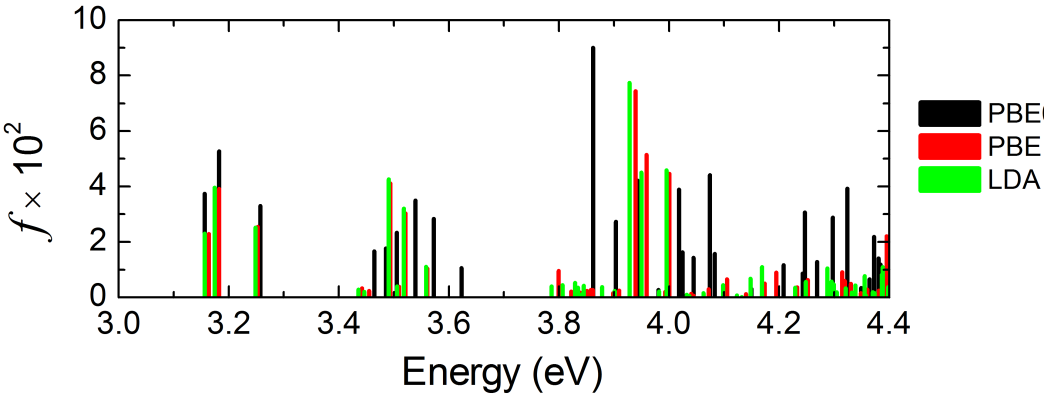


FIG. S1. Oscillator strengths $f$ of optical transitions of the NHC blue emitter at different energies (in eV) calculated using the LDA (green), PBE (red) and PBE0 (black) exchange-correlation functionals. The Casida equation is solved without account of spin-orbit coupling for the isolated complex using the def2-TZVP basis set and def2/J auxiliary basis set. The scissor operators of 0.94 eV and 0.92 eV are applied to the spectra computed using the LDA and PBE functionals, respectively.

[1] D. M. Ceperley and B. J. Alder, "Ground state of the electron gas by a stochastic method," Phys. Rev. Lett. **45**, 566–569 (1980).
[2] J. P. Perdew, K. Burke, and M. Ernzerhof, "Generalized gradient approximation made simple," Phys. Rev. Lett. **77**, 3865–3868 (1996).
[3] C. Adamo and V. Barone, "Toward reliable density functional methods without adjustable parameters: The PBE0 model," J. Chem. Phys. **110**, 6158–6170 (1999).

## MOLECULAR ORBITALS OF EMITTER AND DPBIC

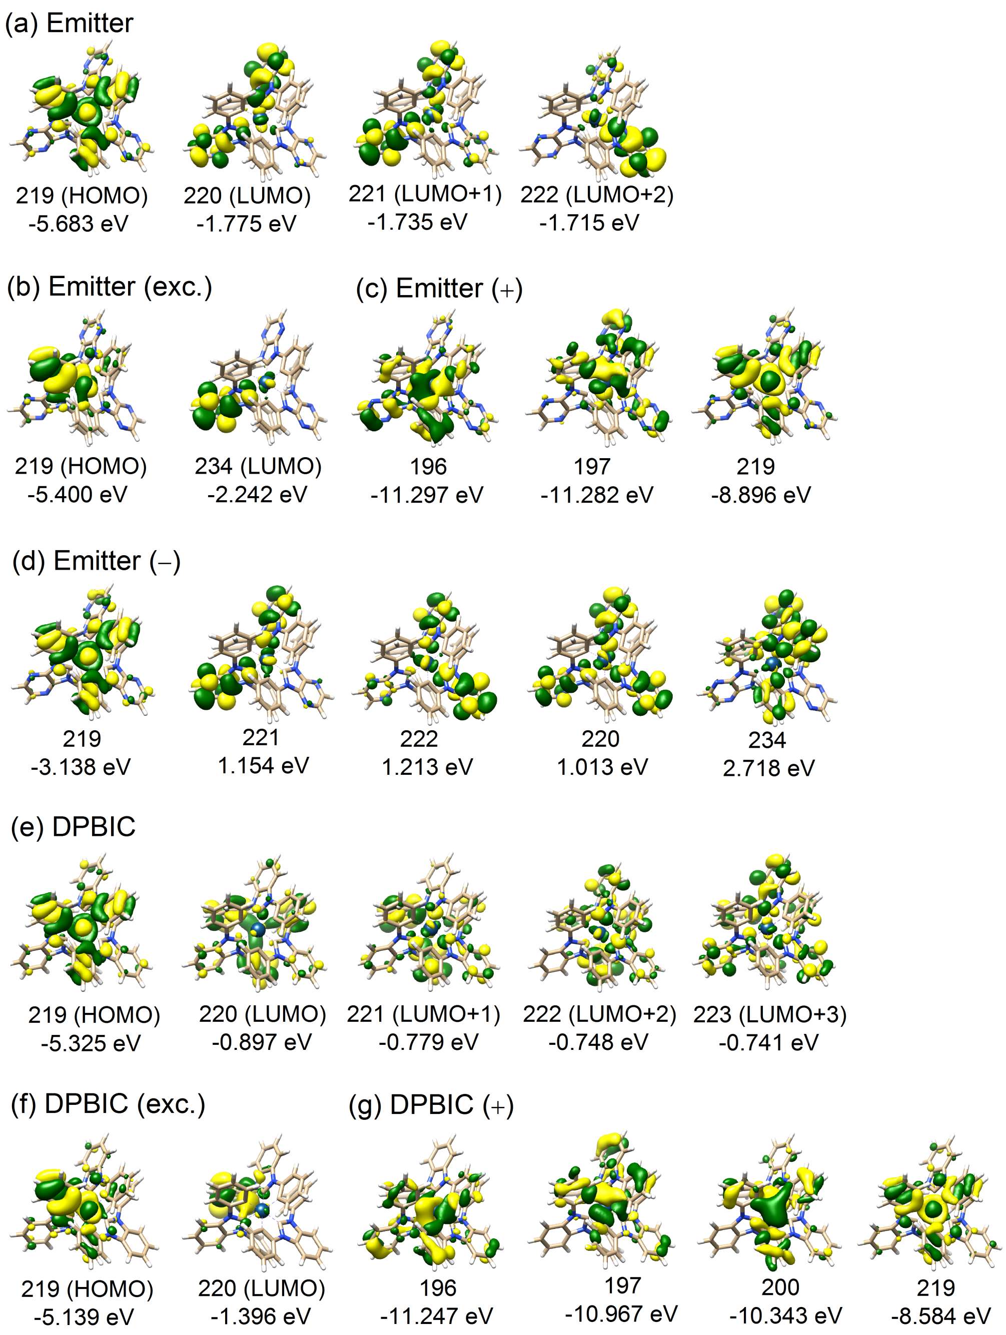


FIG. S2. Contour plots of molecular orbitals for (a) ground-state, (b) excited, (c) positively charged and (d) negatively charged NHC blue emitter and (e) ground-state, (f) excited and (g) positively charged DPBIC. For the neutral species, the orbitals taking part in the lowest-energy transitions are shown. For charged DPBIC, the orbitals taking part in bright excitations close to the emission peak of the NHC dye are included. Isosurfaces correspond to 0.025 Å$^{-3}$. The orbital index and energy are indicated below each orbital. Carbon, nitrogen, hydrogen and iridium atoms are coloured in beige, blue, white and sea blue, respectively. The calculations are performed without account of spin-orbit coupling for the isolated complexes using the PBE0 functional, def2-TZVP basis sets and def2/J auxiliary basis sets.

TABLE S1. Energies $\hbar\Omega$ and transition dipole moments $\mathbf{d}^{\mathrm{T}}$ of singlet excitations computed[a] for neutral, charged and excited organometallic complexes.

| Complex | Charge | $\hbar\Omega$ (eV) | $\lvert\mathbf{d}^{\mathrm{T}}\rvert^2$ (a.u.$^2$) | $d_x^{\mathrm{T}}$ (a. u.) | $d_y^{\mathrm{T}}$ (a. u.) | $d_z^{\mathrm{T}}$ (a. u.) |
|---|---|---|---|---|---|---|
| Blue emitter (excited-state geometry) | 0 | 2.400 | 0.1420 | 0.0012 | -0.3768 | 0.0044 |
| Blue emitter (ground-state geometry) | 0 | 3.156 | 0.4836 | 0.0524 | -0.4055 | -0.5626 |
| | | 3.183 | 0.6751 | 0.0992 | 0.5379 | -0.6132 |
| | | 3.257 | 0.4122 | -0.1808 | -0.4500 | -0.4208 |
| Blue emitter | -1 | 1.825 | 0.3141 | -0.0503 | 0.5316 | -0.1702 |
| | | 1.910 | 0.1968 | 0.0899 | 0.3999 | 0.1696 |
| | | 2.003 | 0.4405 | -0.1892 | -0.0846 | 0.6305 |
| | | 2.238 | 0.0013 | 0.0113 | 0.0283 | -0.0193 |
| | | 2.294 | 0.0019 | 0.0058 | 0.0328 | 0.0282 |
| | | 2.384 | 0.0025 | 0.0110 | 0.0088 | -0.0484 |
| | | 2.477 | 0.0021 | -0.0237 | 0.0261 | -0.0297 |
| | | 2.739 | 0.1742 | -0.1574 | 0.2128 | 0.3227 |
| | | 2.786 | 0.3474 | -0.1855 | -0.5582 | -0.0370 |
| Blue emitter | +1 | 1.906 | 0.1132 | 0.3137 | 0.0164 | -0.1206 |
| | | 1.908 | 0.1934 | 0.0824 | 0.4267 | -0.0672 |
| | | 2.041 | 0.5732 | 0.5766 | 0.4130 | 0.2648 |
| | | 2.203 | 0.0078 | -0.0812 | -0.0321 | 0.0118 |
| | | 2.227 | 0.0641 | 0.1857 | -0.0300 | 0.1696 |
| | | 2.242 | 0.0125 | -0.0912 | -0.0614 | -0.0198 |
| | | 2.256 | 0.0056 | 0.0507 | -0.0503 | -0.0230 |
| | | 2.272 | 0.0672 | 0.1070 | 0.1253 | 0.2002 |
| | | 2.309 | 0.0754 | -0.2621 | -0.0816 | 0.0076 |
| | | 2.365 | 0.0419 | -0.0630 | 0.1574 | 0.1149 |
| | | 2.398 | 0.0544 | -0.0284 | -0.2303 | 0.0222 |
| | | 2.435 | 0.0684 | -0.0093 | 0.0569 | 0.2550 |
| | | 2.599 | 0.0219 | 0.1178 | 0.0897 | -0.0008 |
| | | 2.742 | 0.4938 | -0.0590 | 0.3784 | 0.5892 |
| | | 2.798 | 0.3065 | -0.0730 | 0.3936 | -0.3824 |
| DPBIC | 0 | 3.648 | 0.3171 | -0.0650 | 0.2840 | -0.4819 |
| | | 3.755 | 0.4049 | -0.0470 | 0.4486 | 0.4488 |
| | | 3.784 | 0.1276 | 0.2717 | 0.2308 | 0.0242 |
| | | 3.800 | 0.0458 | -0.0242 | -0.0271 | -0.2109 |
| DPBIC | +1 | 1.943 | 0.2104 | 0.0586 | -0.0574 | 0.4513 |
| | | 1.972 | 0.1878 | -0.3917 | -0.0271 | 0.1834 |
| | | 1.997 | 0.3423 | 0.1799 | 0.5549 | 0.0451 |
| | | 2.231 | 0.0154 | 0.0923 | 0.0828 | 0.0071 |
| | | 2.263 | 0.0068 | -0.0369 | -0.0613 | 0.0404 |
| | | 2.313 | 0.0685 | 0.2536 | -0.0616 | -0.0217 |
| | | 2.390 | 0.2733 | -0.4930 | -0.1129 | -0.1325 |
| | | 2.475 | 0.0452 | -0.0145 | 0.2121 | 0.0019 |
| | | 2.501 | 0.1430 | 0.0211 | 0.2180 | 0.3083 |
| | | 2.552 | 0.0021 | 0.0449 | 0.0090 | 0.0030 |
| | | 2.578 | 0.0459 | -0.0120 | 0.0277 | -0.2122 |
| | | 2.614 | 0.1176 | -0.3192 | -0.1044 | -0.0694 |
| | | 2.671 | 0.0097 | 0.0616 | -0.0497 | -0.0590 |
| | | 2.751 | 0.5082 | 0.0814 | -0.3792 | -0.5981 |
| | | 2.773 | 0.4203 | 0.0433 | -0.4683 | 0.4462 |

[a] Only the most relevant transitions are included. Excitation energies and transition dipole moments are obtained by solving the Casida equation without account of spin-orbit coupling for the isolated complexes using the PBE0 functional, def2-TZVP basis set and def2/J auxiliary basis set.
